# Supplementary material for: Removing supervision in semantic segmentation with local-global matching and area balancing
Source: arXiv:2303.17410 source file (2023-03-30)
Supplement: Supplementary file 1 [file loss_considerations.tex]

In this section, we explore in more detail the motivations behind the apparent fundamental dependence of our method to the OT step and the introduction of the coupling matrices $Q^{\ell}$ and $Q^g$ in Eq. (\textcolor{red}{2}) of the main paper. 

The framework proposed fails when ablating the OT step. In this case, the objective of the minimization problem becomes:
\begin{equation}
    {\mathcal L}_{swap}(P^g,P^{\ell}) = -E_{P^g}[\log P^{\ell}]  - E_{P^{\ell}}[\log P^{g}]
\end{equation}
The above loss has degenerate solutions in both the weakly-supervised and the unsupervised cases. In particular, in the absence of image-level labels, the minimization of ${\mathcal L}_{swap}$ is trivially achieved by assigning each patch to the same cluster, as it is also shown in \cite{asano2019self}. 
This behaviour is partially avoided with weak supervision because ground-truth labels constrain the minimization. However, here a new form of collapse emerges, and the model tends to assign patches to classes in an unbalanced way: for an image with $N$ patches and $k$ classes, $k-1$ patches are assigned to $k-1$ classes while the remaining $N-(k-1)$ patches are assigned to the only class left (usually the background). 

On the other hand, the coupling matrices and the OT step work as an additional constraint to the optimization problem. In practice, we want to replace the cross-entropy terms $-E_{P^g}[\log P^{\ell}]$ with $-E_{q^g}[\log P^{\ell}]$ for some posterior distribution $q_{ij} = q(\text{class}_i| \text{patch}_j)$ which should encode a constraint on how patches are assigned to the $K$ classes. A simple constraint, mimicking \cite{asano2019self, caron2020unsupervised}, would be to enforce $q$ to be a uniform distribution over classes, leading to an objective loss consisting of terms of the type:
\begin{equation}
    \min_{p, q} E_{q}[\log P] \text{ with } q_{ij} = \{0, 1\} \text{ and } \sum_{j=1}^{N} q_{ij} = [\frac{N}{K}, ..., \frac{N}{K}]
\end{equation}
The above condition does not account for variations with respect to object areas. In fact, labels (or pseudo-labels) do not account for how much a certain class covers a particular image. Nevertheless, we can use them, together with our segmentation masks obtained at the previous training step, to estimate what is, on average, the area a particular class occupies in an image of the training set. We can therefore summarize our objective as 
\begin{equation}
    \min_{p, q} E_{q}[\log P] \text{ with } q_{ij} = \{0, 1\} \text{ and } \sum_{j=1}^{N} q_{ij} = \{A_i \nu_i\}_i
\end{equation}
with $A_i$ average occupancy of class $i$ and $\nu_i$ the class frequency in the considered batch.
which is an equivalent formulation of the Optimal Transport problem outlined in the main paper.

A valuable metric to observe to understand how much the model collapses towards degenerate solutions is the intra-class coefficient of variation $c_V$ (defined as the ratio of the standard deviation to the mean) of the area occupied by a specific class across different images. It is straightforward to show that, as we approach a degenerate solution, the coefficient $c_V$ approaches zero. Indeed, when ablating the OT step, we observe that $c_V \xrightarrow[]{} 0 $ very quickly (usually after 2-3 epochs). On the other hand, when employing OT, we avoid collapse and observe that on average $c_V\approx 0.95$.
