# Supplementary material for: Removing supervision in semantic segmentation with local-global matching and area balancing
Source: arXiv:2303.17410 source file (2023-03-30)
Supplement: Supplementary file 2 [file algo.tex]

\vspace*{-0.5cm}
%%%%%%%%%%%%   begin ALGO %%%
\mdfdefinestyle{MyFrame}{%
    linecolor=black,
    outerlinewidth=2pt,
    %roundcorner=20pt,
    innertopmargin=4pt,
    innerbottommargin=4pt,
    innerrightmargin=4pt,
    innerleftmargin=4pt,
        leftmargin = 4pt,
        rightmargin = 4pt
    %backgroundcolor=gray!50!white}
        }
% text
\begin{mdframed}[style=MyFrame,nobreak=true,align=center,userdefinedwidth=24em]
\textbf{Algorithm 1: PC2M in PyTorch pseudo-code}
\end{mdframed}
\vspace*{-0.4cm}
\begin{minted}
[
%frame=lines,
%framesep=2mm,
baselinestretch=1.2,
bgcolor=LightGray,
fontsize=\scriptsize,
mathescape=true
linenos
]
{python}
# f: patch encoder network
# |C|: number of categories
# t: global=g or local=l
# gamma: unit area momentum rate
# eps: scaling value
# nu_D: classes frequencies in dataset
alpha_e = ones(|C|)/|C| 
for e in range(epochs):
  # load minibatch x with b samples and multilabels ll
  for x, ll in loader:
     g = augment(x, crop=false) # preserve global view
     l = augment(x, crop=true) # random views
     pg, pl = f(g), f(l) # patch predictions 
     # pull correct features, push mistaken features
     loss_mce = MCE(ll, pg.max(dim=1)) # GMP
     # classes frequencies in the current batch
     nu_b = ll.sum(dim=0) / ll.sum(dim=(0,1))
     # area distr
     alpha = alpha_e * nu_b / nu_D 
     alpha = alpha / alpha.sum(dim=0)
     kg, kl = kernel(pg,eps), kernel(pl,eps) # stop-gradient
     qg, ql = ot(kg, alpha), ot(kl, alpha) # balance with OT 
     # maximize local-global similarity
     loss_trade = CE(qg, pl)/2 + CE(ql, pg)/2 
     loss = loss_mce + loss_trade 
     loss.backward() # back-propagate
     update(f) # apply gradients

  #offline estimation of unit area rate in epoch e
  q_e = zeros(|C|) # unit area in epoch e 
  for x, ll in loader: 
    q_e += f(x).mean(dim=0) # average category area in x
  # normalize q_e and update unit area rate
  alpha_e = (1-gamma)*alpha_e + gamma*q_e/q_e.sum() 

def CE(q, p):
  # categorical cross-entropy loss
  return - (q * log(p)).sum(dim=1).mean()
  
def MCE(ll, p):
  # multi binary cross entropy loss
  return - (ll * log(p) + (1-ll) * 
               log(1-p)).sum(dim=1).mean()
\end{minted}
%%%%% end algo
